# Supplementary material for: A Learned Closure Method Applied to Phase Mixing in a Turbulent Gradient-Driven Gyrokinetic System in Simple Geometry
Source: arXiv:1912.06769 source file (2021-10-06)
Supplement: Supplementary file 1 [file hp_appendix.tex]

\section{HP Coefficients}
The HP closure coefficients are obtained by matching the frequency response function for the closed N moment system to the exact response function q times in the $\omega \rightarrow 0$ limit - that is the frequency response of the closed system and exact response will match up to $O(\omega^q)$. The resulting closure will have $p=N-2$ closure coefficients. This method is  described in great detail in~\cite{Smith97}. The author shows evidence that the HP closure with $N=4,q=2$ works best. Here we present a short derivation of the HP closure coefficients we use for our system based on the method described in~\cite{Smith97}.

\subsection{Orthogonal Polynomials}
Orthogonal Polynomials:
\begin{equation}
    P_n(x) = P_{n,0}+P_{n,1}x+P_{n,2}x^2 + \dotsc P_{n,n}x^n
\end{equation}
satisfy the following property:
\begin{equation}
    \int_{-\infty}^\infty P_n(x)P_m(x)w(x)dx = \delta_{n,m}
\end{equation}
for a weight function $w(x)$.
They also satisfy the following recurrence relation:
\begin{equation}
    P_n(x) = (a_n x + b_n)P_{n-1}(x) - c_nP_{n-2}(x)
\end{equation}
with coefficients given as follows:
\begin{align*}
    a_n &= \frac{P_{n,n}}{P_{n-1,n-1}},\\
    b_n &=a_n\Big( \frac{P_{n,n-1}}{P_n,n} - \frac{P_{n-1,n-2}}{P_{n-1,n-1}}\Big),\\
    c_n &= \frac{a_n}{a_{n-1}}
\end{align*}

\subsection{The Conjugate Polynomials}
Given $P_n(x)$, the conjugate polynomials $Q_n(x)$ satisfy the same recurrence relation as $P_n(x)$ but have
\begin{equation}
    Q_0(x) = 0,\, Q_1(x) = a_1.
    \label{conjugate_initial}
\end{equation}

The Orthogonal polynomials and their conjugates satisfy the following relation:
\begin{equation}
    P_{n-1}(x)Q_{n}(x) - P_n(x)Q_{n-1}(x) = a_n
    \label{conjugate_relation}
\end{equation}

\subsection{Our Hermites and their Conjugates}
Our Hermite polynomials are defined by:
\begin{equation}
    H_n(x) = \frac{(-1)^ne^{x^2}}{\sqrt{2^n n! \sqrt\pi}}
    \frac{d^n}{dx^n}e^{-x^2}
\end{equation}
And they satisfy 
\begin{equation}
\int_{-\infty}^{\infty} H_{n}(x) H_{m}(x) e^{-x^{2}} d x=\delta_{n, m}
\end{equation}
As well as the recurrence relation:
\begin{equation}
    H_n(x) = \sqrt{\frac{2}{n}} x H_{n-1}(x) - \sqrt{\frac{n-1}{n}}H_{n-2}(x)
    \label{recurrence}
\end{equation}
with 
\begin{equation}
    a_n = \sqrt{\frac{2}{n}},\, b_n = 0,\, c_n = \sqrt{\frac{n-1}{n}}
\end{equation}

The first four Hermite polynomials are shown below:
\begin{align*}
    H_0(x) &= \pi^{-1/4}\\
    H_1(x) &= \sqrt2\pi^{-1/4}\\
    H_2(x) &= \frac{2x^2-1}{\sqrt2\pi^{1/4}}\\
    H_3(x) &= \frac{2x^3 - 3x}{\sqrt3\pi^{1/4}}\\
    H_4(x) &= \frac{4x^4-12x^2+3}{2\sqrt2\sqrt3\pi^{1/4}}
\end{align*}
Choosing these Hermite polynomials as our orthogonal polynomials, i.e. $P_n(x) = H_n(x)$, we can construct the conjugate polynomials using~\ref{conjugate_initial} and~\ref{recurrence} .

The first four conjugate polynomials are shown here:
\begin{align*}
    Q_0(x) &= 0\\
    Q_1(x) &= \sqrt2\, (= a_1)\\
    Q_2(x) &= \sqrt2 x\\
    Q_3(x) &= \frac{2x^2 -2}{\sqrt 3}\\
    Q_4(x) &= \sqrt{\frac{2}{3}}x^3 - (\sqrt{\frac{2}{3}} + \sqrt{\frac{3}{2}})x\\
\end{align*}
\subsection{Conjugate Check}
Now we want to check to make sure our hermites and their conjugates satisfy Eq \ref{conjugate_relation}.
\begin{align*}
n=1:\, P_0Q_1 - P_1Q_0 &= \pi^{-1/4}a_1\,\,\,\,(a_1 = \sqrt 2)\\
n=2:\, P_1Q_2 - P_2Q_1 &= \pi^{-1/4}a_2\,\,\,\,(a_2 = 1)\\
n=3:\, P_2Q_3 - P_3Q_2 &= \pi^{-1/4}a_3\,\,\,\,(a_3 = \sqrt{2/3})\\
n=4:\, P_3Q_4 - P_4Q_3 &= \pi^{-1/4}a_4\,\,\,\,(a_4 = \sqrt{2/4})
\end{align*}
This is where the issue arises. Our Hermites do not satisfy the relationship with the conjugates unless you remove the factor of $\pi^{1/4}$.

\subsection{(N,q)=(4,2) Closure}
\begin{equation}
   R_{00}(\omega) = r_0 + r_1\omega + r_2\omega^2 + \dotsc 
\end{equation}
For the Physicist's Hermite polynomials,
\begin{equation}
    R_{00}(\omega) = -iZ(\omega)
    \label{response}
\end{equation}
where $Z(\omega)$ is the plasma dispersion function.

For our closure we are choosing the $\omega\rightarrow 0$ limit so we can express the plasma dispersion function as this Taylor series:
\begin{equation}
Z(\zeta)=i \sqrt{\pi} e^{-\zeta^{2}}-2 \zeta\left(1-\frac{2 \zeta}{3}+\frac{4 \zeta}{15}-\frac{8 \zeta}{105}+\ldots\right)
\end{equation}
Plugging this in to Eq \ref{response} we get:
\begin{equation}
    R_{00}(\omega) = -i [ i\sqrt\pi e^{-\omega^2} - 2\omega + \dotsc]
\end{equation}
Giving us $r_0 = \sqrt\pi e^{0^2} = \sqrt\pi$ and $r_1 = 2i$

To solve for the closure coefficients $A_3$ and $A_2$ we need to solve the following matrix equation:
\begin{multline}
    \Bigg(\begin{bmatrix}
    r_0 & 0 \\
    r_1 & r_0
    \end{bmatrix}
    \begin{bmatrix}
    P_{3,0} & P_{2,0} \\
    P_{3,1} & P_{2,1}
    \end{bmatrix}
    -i\begin{bmatrix}
    Q_{3,0} & Q_{2,0} \\
    Q_{3,1} & Q_{2,1}
    \end{bmatrix}\Bigg)
    \times\begin{bmatrix}
    A_3\\
    A_2
    \end{bmatrix} \\
    =\begin{bmatrix}
    r_0 & 0 \\
    r_1 & r_0
    \end{bmatrix}
    \begin{bmatrix}
    P_{4,0}\\
    P_{4,1}
    \end{bmatrix}
    -i\begin{bmatrix}
    Q_{4,0}\\
    Q_{4,1}
    \end{bmatrix}
\end{multline}
Plugging in our values for the $P_{i,j},\,Q_{i,j},\, and r_i$ coefficients gives the following matrix equation:
\begin{multline}
    \Bigg(\begin{bmatrix}
    \sqrt\pi & 0 \\
    2i &\sqrt\pi 
    \end{bmatrix}
    \begin{bmatrix}
    0 & -\pi^{-1/4}/\sqrt2 \\
    -\sqrt3\pi^{-1/4} & 0
    \end{bmatrix}\\
    -i\begin{bmatrix}
    -2/\sqrt3 & 0 \\
    0 & \sqrt2
    \end{bmatrix}\Bigg)
    \times\begin{bmatrix}
    A_3\\
    A_2
    \end{bmatrix} \\
    =\begin{bmatrix}
    \sqrt\pi & 0 \\
    2i & \sqrt\pi 
    \end{bmatrix}
    \begin{bmatrix}
    \pi^{-1/4}\sqrt{3}/(2\sqrt2)\\
    0 
    \end{bmatrix}\\
    -i\begin{bmatrix}
    0\\
    -\sqrt{\frac{2}{3}}-\sqrt{\frac{3}{2}} 
    \end{bmatrix}
\end{multline}

Removing the factors of $\pi^{-1/4}$ yields the coefficients $A_3 = -1.75931152j,\, A_2 = 0.75485949$ (same as GX), but including the factors of $\pi^{1/4}$ yields $A_3=+1.11596656j,\, A_2 = -2.23485088 $.
